# Supplementary material for: Spatial fluctuations at vertices of epithelial layers: quantification of regulation by Rho pathway
Source: arXiv:1512.01476 ancillary file (2018-02-06)
Supplement: Supplementary file 1 [file supp3.pdf]

# Supplemental material:

## From motor-induced fluctuations to mesoscopic dynamics in epithelial tissues

É. Fodor,<sup>1,\*</sup> V. Mehandia,<sup>2,3,\*</sup> J. Comelles,<sup>2</sup> R. Thiagarajan,<sup>2</sup> N. S. Gov,<sup>4</sup> P. Visco,<sup>1</sup> F. van Wijland,<sup>1</sup> and D. Riveline<sup>2</sup>

<sup>1</sup>*Laboratoire Matière et Systèmes Complexes, UMR 7057 CNRS/PP7, Université Paris Diderot, 10 rue Alice Domon et Léonie Duquet, 75205 Paris cedex 13, France*

<sup>2</sup>*Laboratory of Cell Physics, ISIS/IGBMC, Université de Strasbourg and CNRS (UMR 7006), 8 allée Gaspard Monge, 67083 Strasbourg, France Development and Stem Cells Program, IGBMC, CNRS (UMR 7104), INSERM (U964), Université de Strasbourg, 1 rue Laurent Fries, BP10142, 67400 Illkirch, France*

<sup>3</sup>*School of Mechanical, Materials and Energy Engineering, Indian Institute of Technology Ropar, India*

<sup>4</sup>*Department of Chemical Physics, Weizmann Institute of Science, 76100 Rehovot, Israel*

(Dated: December 4, 2015)

### I. MATERIALS AND METHODS

#### A. Cell culture and tracking method

We culture cells in DMEM containing 10% Fetal Calf Serum (FCS) and antibiotics. We replate them on glass coverslips (CS) of 25 mm diameter for live cell imaging. When the cell monolayer covered 70% of the CS area, we firmly place the sample at the bottom of a custom made metallic holder. For acquisition, we change the medium to L15, 10% FCS and antibiotics. We use the following inhibitors from myosin activation upstream to Rho: inhibition of acto-myosin by ML7 (Sigma-Aldrich, 10  $\mu$ M), inhibition of Rho kinase (ROCK) by Y-27632 (Sigma-Aldrich, 10  $\mu$ M), and inhibition of Rho by C3 Transferase (Cytoskeleton, 0.04  $\mu$ M). Microtubules are depolymerised with nocodazole (Sigma-Aldrich, 10  $\mu$ M). For observation, we use a motorized inverted microscope (Nikon Eclipse Ti), equipped with a 12 bit CCD camera (Photometric CoolSNAP HQ2). The setup is temperature controlled at 37°C (Life Imaging Services). We check with fluorescent beads (4  $\mu$ m, TetraSpeck) grafted on CS surface that no drift appears during 24 hours of live imaging after 2 hour stabilization. We take pictures of the monolayer every 5 min during the next 8 hours with multiple z-stacks 1  $\mu$ m apart. They span 3  $\mu$ m depth of the cell monolayer. We merge the z-stacks into one image by using the maximum intensity projection. We then extract the vertex positions from the sequence of merged images by manually clicking in each frame as long as they are visible. For each condition, we check that the average cell area was always about  $180 \pm 15 \mu\text{m}^2$ , and we consider more than 20 vertices for at least 3 biological repeats.

#### B. Myosin cluster area and mean intensity

The immunostaining for actin and myosin was performed on wild type MDCK monolayers. After reaching 70-100% confluence, the monolayer was incubated with respective cytoskeletal inhibitor drug for 2 hours and fixed with 3%

paraformaldehyde (PFA). After fixation, the cells were permeabilized with 0.5% Triton in blocking solution (5% BSA solution). The permeabilized samples were treated with 50 mM ammonium chloride solution for 10 minutes at room temperature to quench the auto fluorescence of PFA. For myosin staining, the samples were incubated in rabbit myosin II A non-muscle antibody (Sigma-Aldrich M8064) (1:1000 diluted in blocking solution) for 1 hour. For co-staining actin, the samples were then incubated in a cocktail of Alexa fluor 488 labelled goat anti-rabbit antibody (Molecular Probes A-11034) and Alexa fluor 546 labelled phalloidin (Molecular Probes A-22283) for 1h. Finally the samples were mounted on microscope slide with glycerol-PBS (1:1) mixture for imaging.

Fluorescence images of actin and myosin throughout the monolayer were acquired through z-stacks by using a Cool-Snap HQ2 camera mounted on a Nikon Ti epifluorescence microscope with a x60 oil objective. Apical myosin structures were identified, their area and mean intensity were measured using Image J. Values were normalized to the mean cluster intensity of control condition from each biological repeat. Statistics (N: number of experiments, n: number of clusters): (i) control N=2, n=312; (ii) myosin inhibitor N=2, n=186; (iii) rho kinase inhibitor N=2, n=197; (iv) rho inhibitor N=2, n=257; (v) depolymerized microtubule N=2, n=111.

#### C. Cell area measurement and E-cadherin intensity

Cell boundaries were identified and cell area was measured. A polygon was assigned to the area and the boundary of each cell using Packing Analyzer software [1–4]. Statistics (N: number of experiments, n: number of cells): (i) control N=4, n=235; (ii) myosin inhibitor N=4, n=246; (iii) rho kinase inhibitor N=3, n=249; (iv) rho inhibitor N=3, n=148; (v) depolymerized microtubule N=4, n=243.

Afterwards, the segmented images identifying cell boundaries were used as mask for E-cadherin intensity. The boundaries were dilated up to 7 pixels using Image J. The resulting image was applied as mask on the original GFP-E-cadherin image. Statistics (N: number of experiments, n: number of contacts): (i) control N=4, n=311; (ii) myosin inhibitor N=4, n=566; (iii) rho kinase inhibitor N=4, n=555; (iv) rho inhibitor N=2, n=339; (v) depolymerized microtubule N=4, n=357.

\* These authors contributed equally to this work

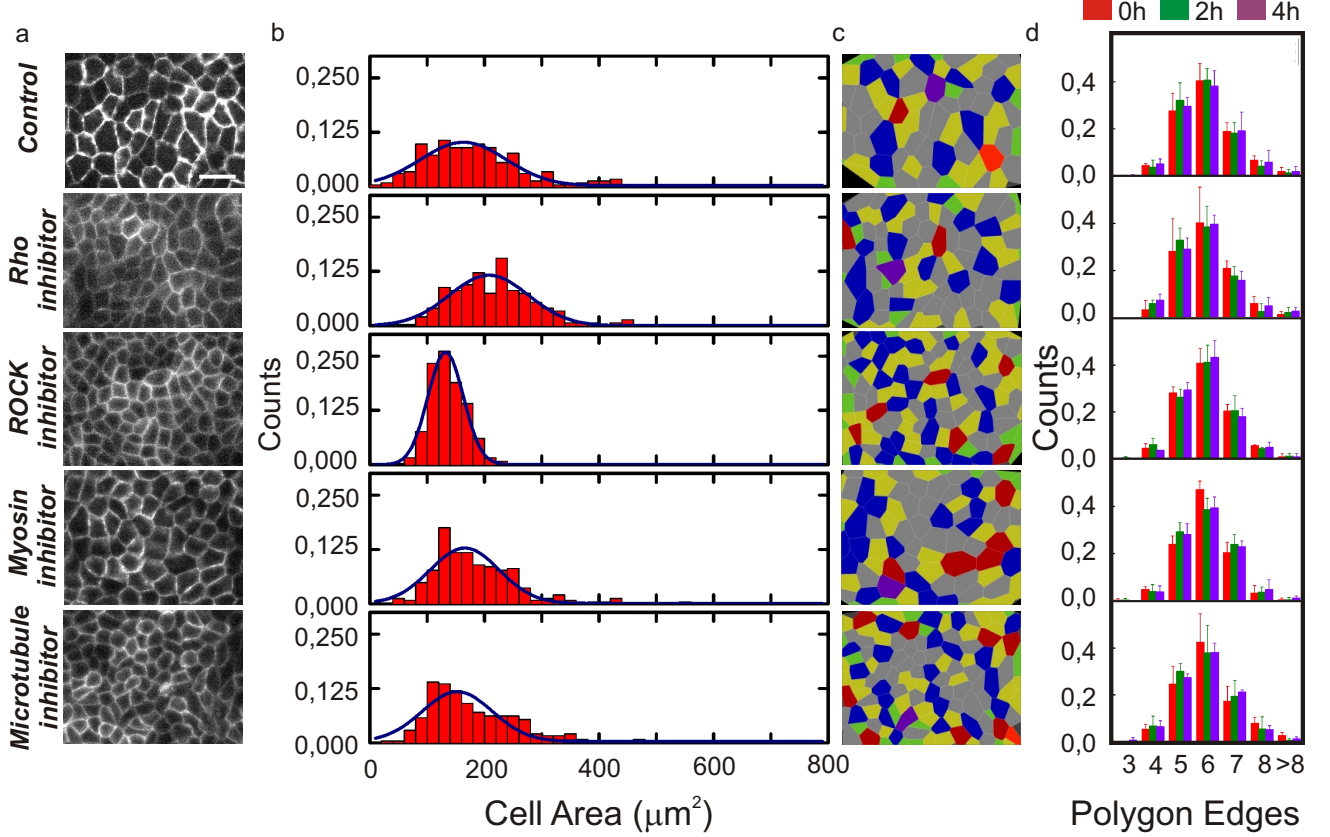

FIG. S1. (Color online) Monolayer architecture. (a) Snapshots of cell-cell contacts (GFP-E-cadherin) for each condition after 4 hours. Scale bar 20  $\mu\text{m}$ . (b) Histograms of single cell area after 4 hours for each condition. (c) Polygon approximation of (a). (d) Distribution of polygons at 0, 2 and 4 hours.

## II. CAGING MODEL

### A. Presentation

We consider the following set of equations for the two-dimensional positions of the vertex  $\mathbf{r}$  and the cage center  $\mathbf{r}_0$

$$\gamma \frac{d\mathbf{r}}{dt} = -k(\mathbf{r} - \mathbf{r}_0) + \sqrt{2\gamma k_B T} \boldsymbol{\xi}, \quad \frac{d\mathbf{r}_0}{dt} = \mathbf{v}_A, \quad (\text{S1})$$

where  $\boldsymbol{\xi}$  is a zero mean isotropic Gaussian white noise, and  $\mathbf{v}_A$  is a stochastic process consisting in alternating active phases with quiescent periods. The bath temperature is denoted by  $T$ , and  $\gamma$  is the friction coefficient. In the active phase,  $\mathbf{v}_A$  has a constant value  $v$  over a random direction uniformly sampled in the two-dimensional space during an exponentially distributed time of average  $\tau$ . In the quiescent phase,  $\mathbf{v}_A = \mathbf{0}$  during an exponentially distributed time of mean value  $\tau_0$ .

The projection of the process  $\mathbf{v}_A$  on one dimension defines the process  $v_A$ . We denote  $P_{2D}$  and  $P_{1D}$  the distributions of a two-dimensional unit vector  $\hat{\mathbf{n}}$ , and of  $n_x = \hat{\mathbf{n}} \cdot \hat{\mathbf{x}}$  in the  $x$ -axis, respectively. They are related as  $P_{2D}(\theta) |d\theta| = P_{1D}(n_x) |dn_x|$ , where  $\hat{\mathbf{n}} = (\cos \theta, \sin \theta)$  in the  $(x, y)$  basis. Given  $P_{2D} = 1/(2\pi)$  is uniform and  $n_x = \cos \theta$ , we deduce

$P_{1D} = |d \arccos(n_x)/dn_x|/(2\pi)$ . It follows that the active phase of  $v_A$  is now characterized by a random velocity in the interval  $[-v, v]$  distributed as

$$P(v_A) = \frac{1}{\pi v \sqrt{1 - (v_A/v)^2}}. \quad (\text{S2})$$

The time distribution of each phase remains unchanged in the projected process. From this result, we arrive at the equations for the projected positions  $x$  and  $x_0$

$$\gamma \frac{dx}{dt} = -k(x - x_0) + \sqrt{2\gamma k_B T} \xi, \quad \frac{dx_0}{dt} = v_A, \quad (\text{S3})$$

where  $\xi$  is still a zero mean Gaussian noise such as  $\langle \xi(t) \xi(t') \rangle = \delta(t - t')$ , and now  $v_A$  is the random process depicted in Fig. S3. It is a zero mean non-Gaussian colored noise with correlations  $\langle v_A(t) v_A(t') \rangle = D_A e^{-|t-t'|/\tau}/\tau$ , where  $D_A = (v\tau)^2/[2(\tau + \tau_0)]$  defines an active diffusion coefficient in terms of the active parameters.

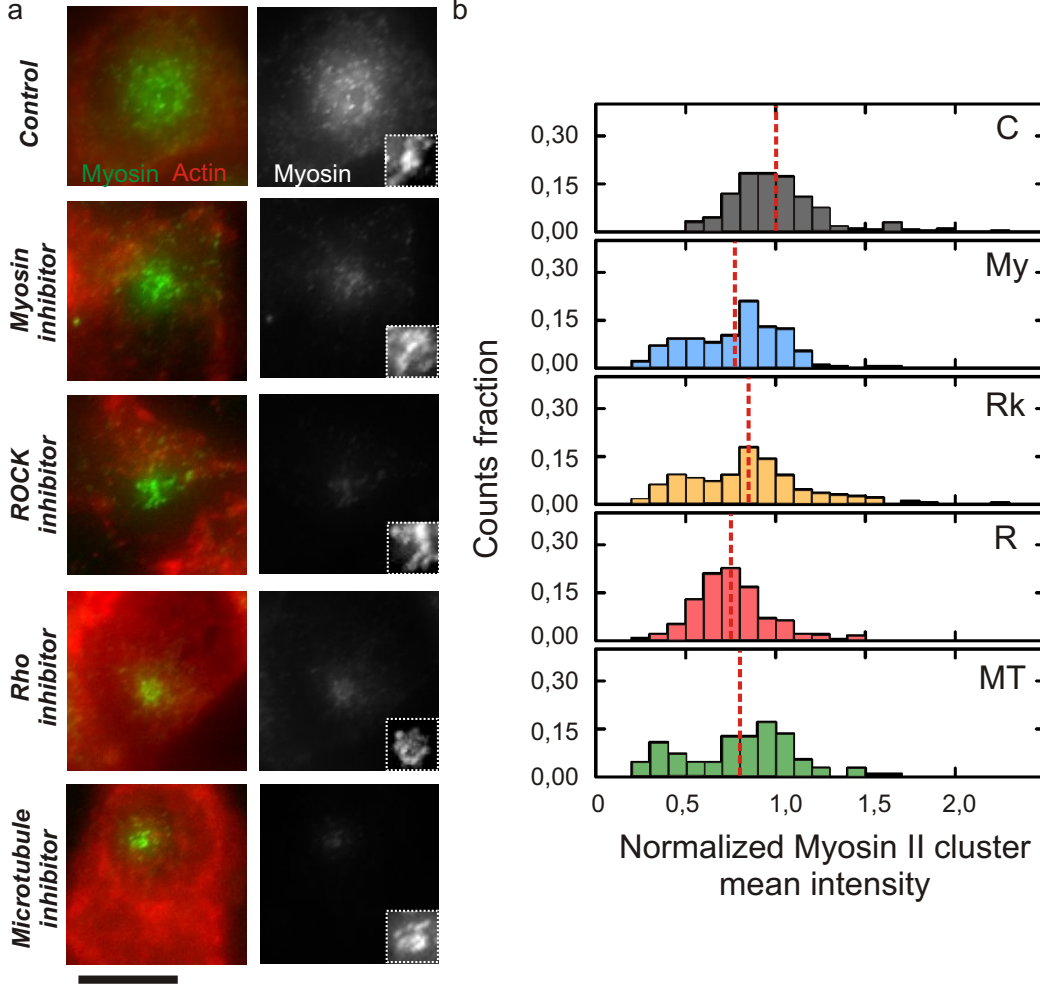

FIG. S2. (Color online) Acto-myosin cytoskeleton. (a) Actin (red) and myosin (green) structures, and (b) myosin structure alone at the apical surface of MDCK cells for the different experimental conditions. Scale bar is  $5 \mu\text{m}$ . The Lookup Table (LUT) were unaltered to show the differences in actin and myosin intensities. Insets in (b) show zooms on typical myosin clusters with increased contrast for clarity. (c) Distributions of myosin clusters mean intensity for each condition after 2 hours of the beginning of the experiment. Values were normalized to the mean cluster intensity of control condition from each biological repeat. The dashed red lines indicate the mean value.

### B. Analogy with active cell-cell junctions

We consider that a cell-cell junction acts as a spring on the vertex. We treat the fluctuations of these junctions with an active noise regulating the dynamics of the rest length of the associated spring. We account for the interaction with the surrounding bath by means of a white noise term and a damping force, and we discard inertial effects. It follows that the dynamics of the vertex position  $\mathbf{r}$  obeys

$$\gamma \frac{d\mathbf{r}}{dt} = -k(3\mathbf{r} - \mathbf{r}_1 - \mathbf{r}_2 - \mathbf{r}_3) + \boldsymbol{\xi}, \quad \frac{d\mathbf{r}_i}{dt} = \mathbf{v}_{Ai}, \quad (\text{S4})$$

where  $\mathbf{r}_i$  denotes the position of each neighboring vertex and where each noise term  $\mathbf{v}_{Ai}$  has the same properties as  $\mathbf{v}_A$  defined above, with zero cross correlations. By projecting Eq. (S4) on one dimension, we end up with a dynamics sim-

ilar to Eq. (S3), where the correlations of the noise term  $v_A$  exhibit the same exponential decay.

### C. Mean square displacement

From the Fourier transform of Eq. (S3), we compute the position autocorrelation function  $C(t) = \langle x(t)x(0) \rangle$ , and then deduce the one-dimensional mean square displacement (MSD) as  $\langle \Delta x^2 \rangle(t) = 2(C(0) - C(t))$ . We denote the thermal contribution to the MSD by  $\langle \Delta x_T^2 \rangle$ , and the MSD when the particle is only subjected to motor activity by  $\langle \Delta x_A^2 \rangle$ , so that:  $\langle \Delta x^2 \rangle = \langle \Delta x_T^2 \rangle + \langle \Delta x_A^2 \rangle$ . The thermal MSD is the same as for an Ornstein-Uhlenbeck process, and we compute the active contribution in terms of the parameters characteriz-

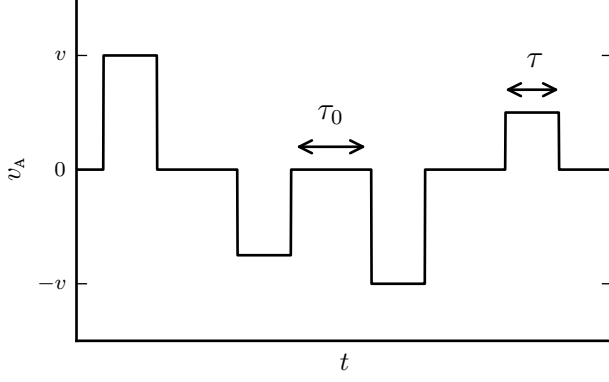

FIG. S3. Example trajectory of the active burst projection  $v_A$ . It equals zero over a random duration of average  $\tau_0$ , and is a random value between  $-v$  and  $v$  during a random time of order  $\tau$ .

ing the active force

$$\langle \Delta x_T^2 \rangle(t) = 2D_T \tau_T \left(1 - e^{-t/\tau_T}\right), \quad (\text{S5a})$$

$$\langle \Delta x_A^2 \rangle(t) = \frac{2D_A \tau_r}{1 - (\tau/\tau_r)^2} \left[ \left(\frac{\tau}{\tau_r}\right)^3 \left(1 - e^{-t/\tau} - \frac{t}{\tau}\right) + e^{-t/\tau_r} + \frac{t}{\tau_r} - 1 \right], \quad (\text{S5b})$$

where  $D_T = k_B T / \gamma$  is the thermal diffusion coefficient, and  $\tau_r = \gamma / k$  is a microscopic relaxation time scale. It appears the MSD depends on four independent parameters, two of them characterizing active fluctuations  $\{D_A, \tau\}$ , and the two others being associated with equilibrium thermal properties  $\{D_T, \tau_r\}$ .

### III. DATA ANALYSIS

#### A. Mean square displacement

We extract the experimental MSD from individual trajectories in each condition. We compute the value of the MSD at each time  $t$  by performing a sliding time average on every trajectory, and an ensemble average over the different trajectories

$$\text{MSD}(t) = \frac{\Delta t}{N(t_m - t)} \sum_{j=1}^N \sum_{i=1}^{\frac{t_m - t}{\Delta t}} [x_j(t + i\Delta t) - x_j(i\Delta t)]^2, \quad (\text{S6})$$

where  $N$  is the number of experimental trajectories,  $t_m = 8$  hours is the longest measurement time, and  $\Delta t = 5$  min is the experimental sampling time. The error bars for the estimated active parameters shown in Fig. 2 of the main text account for the standard error of the experimental points. These errors are used as weights associated with each point in the average MSD when fitting the experimental data. Moreover, we report a systematic error due to the spatial resolution, which we estimate as  $0.2 \mu\text{m}$ .

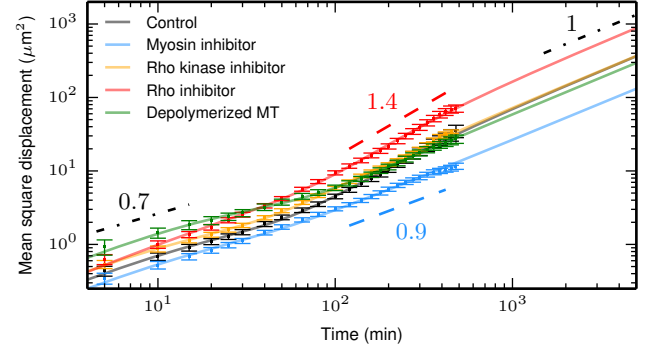

FIG. S4. (Color online) Mean square displacement as a function of time in five conditions: control (black), myosin inhibitor (blue), Rho kinase inhibitor (orange), Rho inhibitor (red), and microtubule depolymerization (green). The corresponding best fitting curves are in solid lines. The best fit curves are extended beyond the experimental time window to highlight the predicted large time diffusive regime.

We present in Fig. S4 the MSD data for the five conditions along with the best fit curves for which we have extended the time window with respect to Fig. 2(a) in the main text, thus highlighting the predicted large time diffusive regime.

#### B. T1 transition

We analyse a vertex trajectory which contains a T1 transition, that is for which two neighbouring vertices merge during the trajectory (Fig. S5). To provide a quantitative probe of the merging event, we compute the vertex interdistance as a function of time. We identify the time interval of the T1 transition as the time needed for the two vertices to gather and then separate. In that respect, we assume that the transition ends when the vertex interdistance increases again. The interdistance fluctuates around  $15 \mu\text{m}$  until about 300 min when it starts to drop off, and it increases again at  $\sim 600$  min.

We extract the MSD of the trajectory by performing an ensemble average only over the neighbouring vertices. The MSD exponent is close to 1 at short and large times, that is before and after the transition. During the transition, the exponent first increases rapidly, and then decreases to reach a ballistic regime until the end of the transition. This behavior supports the hypothesis that T1 transitions correspond to superdiffusive events in the vertex trajectory, which are triggered by active fluctuations within our model.

### IV. NUMERICAL SIMULATIONS

#### A. Methods

We use Euler's method to simulate Eq. (S3). The iterative equations take the following form in terms of the sampling

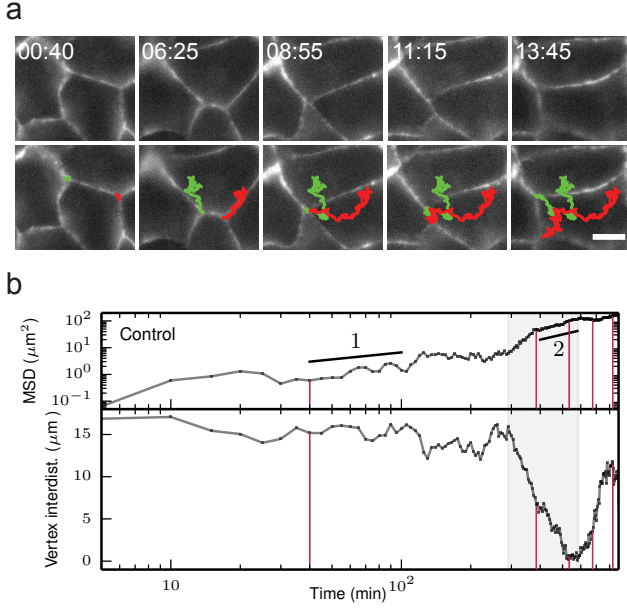

FIG. S5. (Color online) (a) Snapshots of a vertex undergoing a T1 transition, visualized by GFP-E-Cadherin. Red and green lines describe the trajectories of triple points during a T1 transition. Time in hh:mm. Scale bar  $10 \mu\text{m}$  (see movie in [5]). (b) Plot of the evolution of the mean square displacement (MSD) and vertex inter-distance for the T1 transition shown in (a). Black lines are guides to eyes for the diffusive and superdiffusive regimes. Vertical red lines correspond to the time points of snapshots in (a).

time  $\Delta t$

$$x(t + \Delta t) = x(t) - \frac{\Delta t}{\tau_r} (x(t) - x_0(t)) + \sqrt{2D_r \Delta t} \eta, \quad (\text{S7a})$$

$$x_0(t + \Delta t) = x_0(t) + v_A(t) \Delta t, \quad (\text{S7b})$$

where  $\eta$  is a random Gaussian variable with zero mean and variance 1. The iterative equation for the active burst  $v_A$  obeys

$$v_A(t + \Delta t) = \begin{cases} v_A(t) & \text{if } v_A(t) \neq 0 \text{ prob. } 1 - \Delta t/\tau, \\ v_A(t) & \text{if } v_A(t) = 0 \text{ prob. } 1 - \Delta t/\tau_0, \\ 0 & \text{if } v_A(t) \neq 0 \text{ prob. } \Delta t/\tau, \\ \chi_{[-v,v]} & \text{if } v_A(t) = 0 \text{ prob. } \Delta t/\tau_0, \end{cases} \quad (\text{S8})$$

where  $\chi_{[-v,v]}$  is a random number between  $-v$  and  $v$  with probability given by Eq. (S2).

## B. Results: Short-time dynamics

We extract the probability distribution function (PDF) of displacement from the simulated trajectories, to be compared with the experimental distributions. The short time dynamics is Gaussian and entirely controlled by the passive parameters

$\{D_r, \tau_r\}$ . First, we run simulations with the best values estimated from the fit of the experimental MSD, as reported in Tab. I, without any active noise, namely  $v_A = 0$ . The corresponding PDFs reproduce the experimental data, as shown in Fig. S6(a-e). Then, we include the active nonequilibrium fluctuations. The short time PDF is still Gaussian as expected, and we adjust the value of  $v\tau$  by matching the exponential tails between numerical results and experimental data (Fig. 2(b-f) of the main text). We present in Fig. S6(f) the comparison between the analytic MSD in Eq. (S5) and the MSD extracted from simulated trajectories, showing a good agreement. This confirms that there is a well defined time scale which separates equilibrium fluctuations from active nonequilibrium fluctuations.

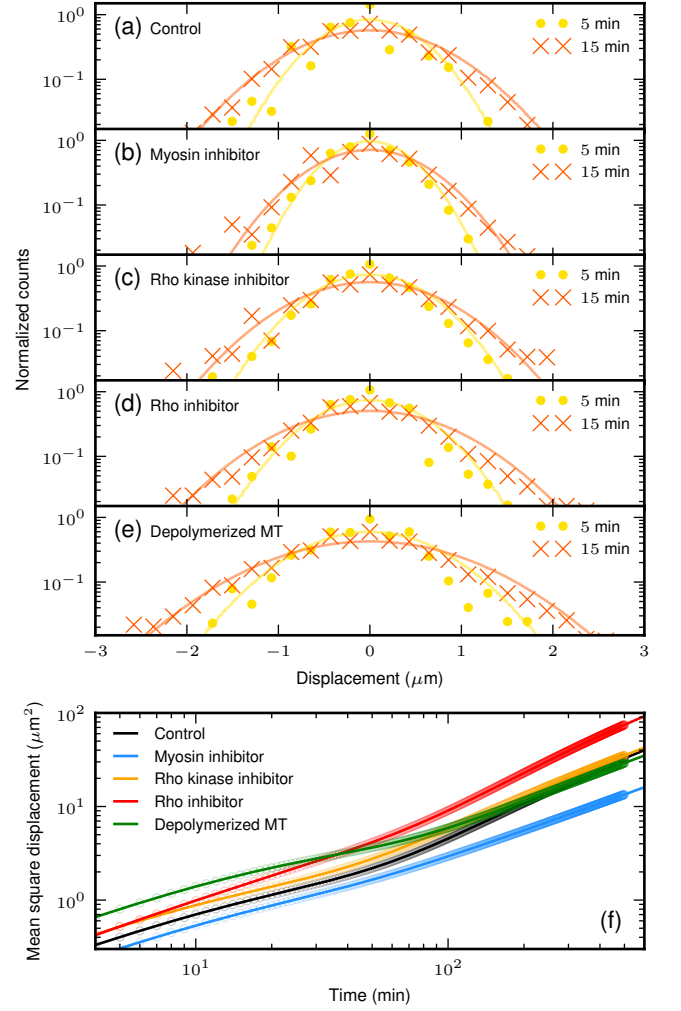

FIG. S6. (Color online) (a-e) Probability distribution function of displacement for the five conditions at two times: 5 (yellow ●), and 15 min (orange ×). We present the results of simulations without active noise of the vertex dynamics in solid lines. (f) Mean square displacement as a function of time in five conditions: control (black), myosin inhibitor (blue), Rho kinase inhibitor (orange), Rho inhibitor (red), and microtubule depolymerization (green). Results of simulations with active noise are shown in ○, and the corresponding analytic curves are in solid lines.

TABLE I. Best fit value of  $D_T$  and  $\tau_T$  estimated from the fit of the experimental MSD presented in Fig. 2(a) of the main text.

|                 | $D_T$ ( $10^{-2} \mu\text{m}^2/\text{min}$ ) | $\tau_T$ (min) |
|-----------------|----------------------------------------------|----------------|
| Control         | $2.4 \pm 0.2$                                | $13 \pm 2$     |
| Myosin inh.     | $1.8 \pm 0.1$                                | $13 \pm 3$     |
| Rho kinase inh. | $3.2 \pm 0.2$                                | $10 \pm 1$     |
| Rho inh.        | $2.8 \pm 0.2$                                | $24 \pm 6$     |
| Depolym. MT     | $4.6 \pm 0.7$                                | $15 \pm 4$     |

- 
- [1] M. C. Gibson, A. B. Patel, R. Nagpal, and N. Perrimon, [Nature](#) **442**, 1038 (2006).
- [2] R. Farhadifar, J.-C. Röper, B. Aigouy, S. Eaton, and F. Jülicher, [Current Biology](#) **17**, 2095 (2007).
- [3] B. Aigouy, R. Farhadifar, D. B. Staple, A. Sagner, J.-C. Röper, F. Jülicher, and S. Eaton, [Cell](#) **142**, 773 (2010).
- [4] D. Staple, R. Farhadifar, J.-C. Röper, B. Aigouy, S. Eaton, and F. Jülicher, [EPJE](#) **33**, 117 (2010).
- [5] See Supplemental Material at [URL will be inserted by publisher] for a movie of a typical T1 transition. Scale bar is  $10 \mu\text{m}$ , time is in hh:mm; red and blue points record vertex trajectories.
